# Supplementary material for: Chirality induced Giant Unidirectional Magnetoresistance in Twisted Bilayer Graphene
Source: arXiv:2010.08385 source file (2021-02-02)
Supplement: Supplementary file 1 [file SM.pdf]

In this Supplemental Information we present a proof that the UMR vanishes in the absence of dephasing for a two-terminal setup. Furthermore, data is presented for the UMR for several twist angles, illuminating the dependence of the effect on the parameters $L$ and $\eta$. Finally, we elucidate some details of the semiclassical approach.

## S1. PROOF OF $\Delta G = 0$ FOR TWO-TERMINAL TRANSPORT WHEN $\eta = 0$

For a two-terminal system the conductance from lead $i$ to $j$ ($i, j = 1, 2$) is $G_{j\leftarrow i} = \mathrm{Tr}(\Gamma_j \mathcal{G} \Gamma_i \mathcal{G}^\dagger)$ in units of $e^2/h$, where $\Gamma_{i,j} = i(\Sigma_{i,j} - \Sigma_{i,j}^\dagger)$ is the anti-Hermitian part of the self-energy $\Sigma_{i,j}$. $\mathcal{G}$ is the (retarded) Green function of the scattering region defined as $\mathcal{G}^{-1} = (E + i\eta)I - H - (\Sigma_1 + \Sigma_2)$, where $I$ is the identity matrix, and $H$ is the tight-binding Hamiltonian. The total self-energy is the sum of the two leads $\Sigma = \Sigma_1 + \Sigma_2$. When $\eta = 0$, we have

$$\mathcal{G}^{-1} - (\mathcal{G}^\dagger)^{-1} = -\Sigma + \Sigma^\dagger = i\Gamma. \tag{S1}$$

Multiplying Eq. (S1) with $\mathcal{G}$ and $\mathcal{G}^\dagger$ as $\mathcal{G}\times$ (S1) $\times\mathcal{G}^\dagger$ and $\mathcal{G}^\dagger\times$ (S1) $\times\mathcal{G}$, respectively, we have

$$\begin{aligned} \mathcal{G}^\dagger - \mathcal{G} &= i\mathcal{G}\Gamma\mathcal{G}^\dagger = i\mathcal{G}^\dagger\Gamma\mathcal{G}, \\ \Gamma &= \Gamma_1 + \Gamma_2. \end{aligned} \tag{S2}$$

Here, the first line follows if $\eta = 0$, while the second line is a result of the two-terminal structure. Therefore

$$\begin{aligned} \Delta G &= G_{2\leftarrow 1} - G_{1\leftarrow 2} \\ &= \mathrm{Tr}(\Gamma_2\mathcal{G}\Gamma_1\mathcal{G}^\dagger) - \mathrm{Tr}(\Gamma_1\mathcal{G}\Gamma_2\mathcal{G}^\dagger) \\ &= \mathrm{Tr}(\Gamma\mathcal{G}\Gamma_1\mathcal{G}^\dagger) - \mathrm{Tr}(\Gamma_1\mathcal{G}\Gamma\mathcal{G}^\dagger) \\ &= \mathrm{Tr}(\Gamma_1\mathcal{G}^\dagger\Gamma\mathcal{G}) - \mathrm{Tr}(\Gamma_1\mathcal{G}\Gamma\mathcal{G}^\dagger) \\ &= 0 \end{aligned} \tag{S3}$$

Thus in order to have nonzero $\Delta G$ we must either introduce finite dephasing or use multi-terminal structure.

## S2. DEPENDENCE OF PEAK VALUE OF $\Delta G/G_0$ ON $L$ AND $\eta$

The relative change of conductance $G$ is defined as

$$P = \frac{\Delta G}{G_0} = \frac{G_2 - G_1}{G_2 + G_1}, \tag{S4}$$

where $G_1$ and $G_2$ are the conductances for opposite current directions. Let $x = \eta L/\hbar$, then $G_{1,2}$ can be expressed as

$$G_{1,2} = \frac{e^2}{h}\sum_n \frac{1}{1 + (x/v_{1,2}^{(n)})}, \tag{S5}$$

where $n$ labels different transport modes. $P$ equals 0 when $x \to 0$ because the numbers of modes for two opposite transport directions are the same. For small but finite $x$, $\frac{1}{1+(x/v)} \approx 1 - (x/v)$. Thus

$$P \approx \frac{\sum_n[1 - (x/v_2^{(n)})] - \sum_n[1 - (x/v_1^{(n)})]}{\sum_n[1 - (x/v_2^{(n)})] + \sum_n[1 - (x/v_1^{(n)})]} \approx \frac{x}{2N}\sum_n\left(\frac{1}{v_1^{(n)}} - \frac{1}{v_2^{(n)}}\right), \tag{S6}$$

where N is the total number of modes. Therefore for small $x$, $P$ increases linearly with $x$. When $x \to +\infty$, we have $\frac{1}{1+(x/v_{1,2}^{(n)})} \approx \frac{1}{x/v_{1,2}^{(n)}} = \frac{v_{1,2}^{(n)}}{x}$, thus

$$P = \frac{\sum_n v_2^{(n)} - v_1^{(n)}}{\sum_n v_2^{(n)} + v_1^{(n)}} \tag{S7}$$

which is independent of $x$. The changing rate of $P$ with respect to $x$ is

$$P' = \frac{2G_2'G_1 - 2G_1'G_2}{(G_2 + G_1)^2} = \frac{2G_1G_2}{(G_1 + G_2)^2}(G_2'/G_2 - G_1'/G_1). \tag{S8}$$

In the case of single mode input and output, $P'$ is always positive because

$$\frac{G_2'}{G_2} - \frac{G_1'}{G_1} = \frac{-1}{v_2 + x} - \frac{-1}{v_1 + x} = \frac{v_2 - v_1}{(v_2 + x)(v_1 + x)} > 0. \tag{S9}$$

Thus for single mode transport, $P$ first increases with $x$ and then saturates. For the multimode case $P$ first increases to a peak value and then decreases, approaching a constant value.

## S3. SEMICLASSICAL MODEL OF RELAXATION

The following considerations are perturbative in the dephasing rate $\eta$. We start with the assumption that the current relaxes either directly between left- and right-mover with a rate $\frac{1}{\tau} \propto \eta$ or indirectly via intermediate steps involving states from other bands. This latter case presents an additional relaxation path which contributes additively with a rate $\frac{1}{\tau_i} \propto \eta$ to the total momentum relaxation rate. To leading order in $\eta$, the corrected relaxation rate is thus $\frac{1}{\tau} + \frac{1}{\tau_i}$. Because $\tau_i$ involves intermediate states, the total rate may of course receive higher-order corrections from subsequent relaxation processes to the ground state. We emphasize that this approach is not related to the usual calculation of the conductivity due to impurity scattering, phonons or interactions, which would involve the determination of the transport time from Kubo's formula. While this procedure precisely leads to a finite dephasing $\eta$, it only involves relaxation processes within the same band. The effect discussed here of the opening of a weak side channel of relaxation is instead a result of the weak but finite transition matrix element that allows inelastic transitions between different bands, which becomes possible thanks to the finite $\eta$. As a consequence, the momentum loss due to the side channel is generically much smaller, i.e. $\tau_i \gg \tau$, meaning that the resulting correction to the relaxation rate and the conductivity could be disregarded if it weren't the leading contribution to $\Delta G$. In summary, Eqs. (2,3) of the main text hold perturbatively for small $\eta$. Most importantly, they can hold even if $\eta L \to \infty$.

In the opposite limit of large $\eta$, the previous perturbative arguments must fail. Since both $\tau_i$ and $\tau$ become very small, it becomes reasonable to consider the secondary relaxation channel with lifetime $\tau_i$ as a way to store some momentum in intermediate states, instead of completely relaxing it with lifetime $\tau$. We thus expect the total momentum lifetime to *increase* to $\tau + \tau_i$ in the presence of a side channel. In terms of $\tau$, we therefore suggest for the conductivity the form

$$\Delta G \propto \frac{\tau}{1 + \frac{\tau^2}{\tau_0^2}}, \tag{S10}$$

where $\tau_0$ is an intermediate scale where the primary relaxation path becomes comparable to the side channel. Importantly, we do not imply that such a relation should hold in terms of $\eta$, because the precise relation between $\tau$ and $\eta$ is not known for all values of $\eta$. Indeed, from the calculations using the NEGF method, we recover that $\Delta G \to 0$ for large $\eta$, but the decay does not follow the prescription $\tau \sim 1/\eta$.

For the parameters considered in the main text, the precise form of the decay of $\Delta G$ at large $\eta$ is immaterial, but we point out that the limiting value of $\Delta G$ [Eq.(S7)] as calculated in the perturbative picture might not be visible in all systems, depending on the microscopic processes which lead to a finite $\eta$.

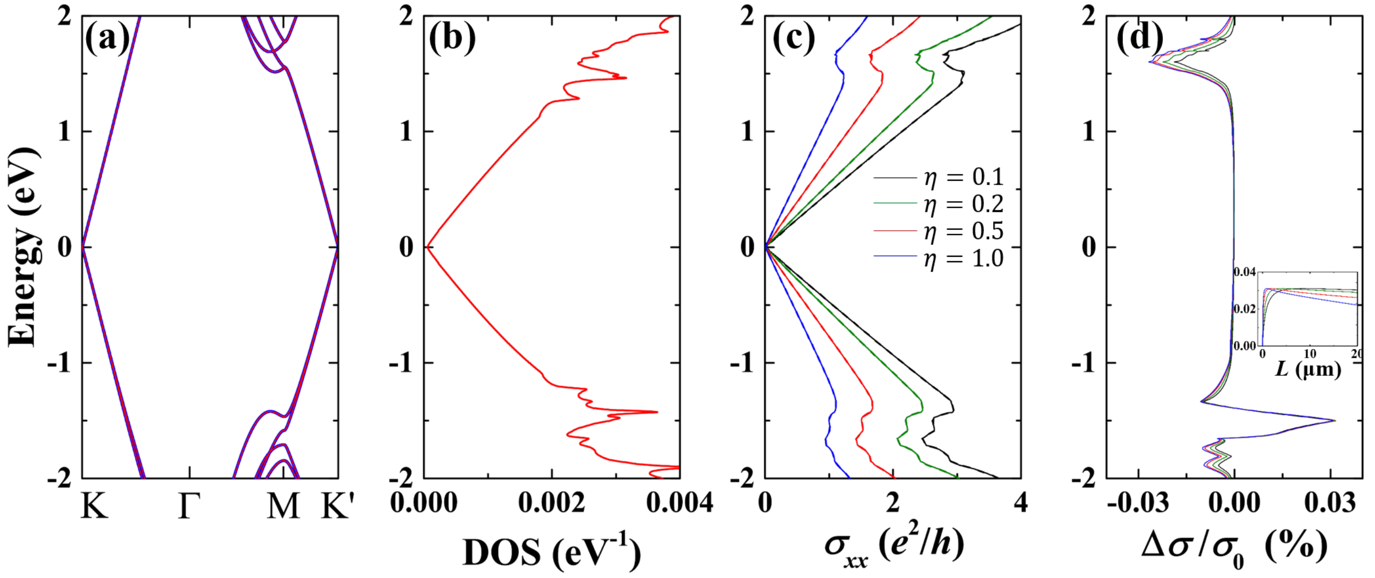


FIG. S1: **At twist angle $\theta$= 21.8°.** (a) Band structure, (b) density of states (DOS), (c) conductivity $\sigma_{xx}$, and (d) relative change of $\sigma_{xx}$ of TBG for **I** || **B** (B=10 T) as functions of energy for fixed length $L = 2\mu$m. In (c)-(d) the black, green, red, and blue lines are calculated under dephasing $\eta = 0.1, 0.2, 0.5$, and 1.0 meV, respectively. The inset in (d) shows the length dependence of the positive peak value under fixed dephasing $\eta = 1$ meV.

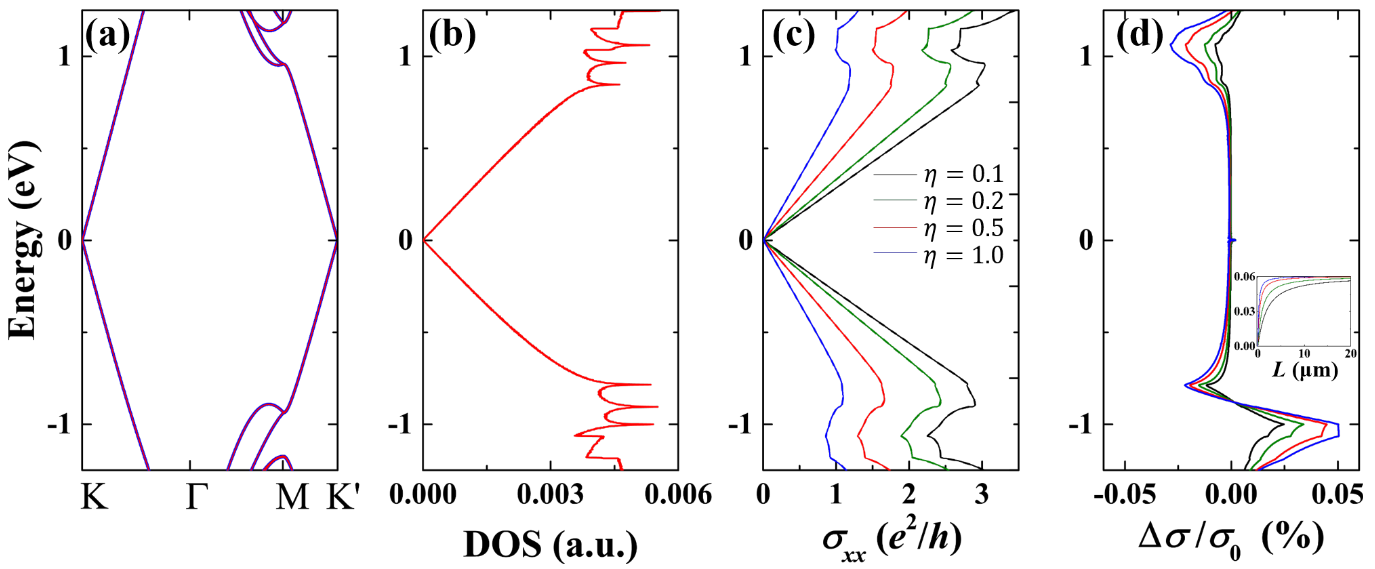


FIG. S2: **At twist angle $\theta$= 13.2°.** (a) Band structure, (b) density of states (DOS), (c) conductivity $\sigma_{xx}$, and (d) relative change of $\sigma_{xx}$ of TBG for **I** || **B** (B=10 T) as functions of energy for fixed length $L = 2\mu$m. In (c)-(d) the black, green, red, and blue lines are calculated under dephasing $\eta = 0.1, 0.2, 0.5$, and 1.0 meV, respectively. The inset in (d) shows the length dependence of the positive peak value under fixed dephasing $\eta = 1$ meV.

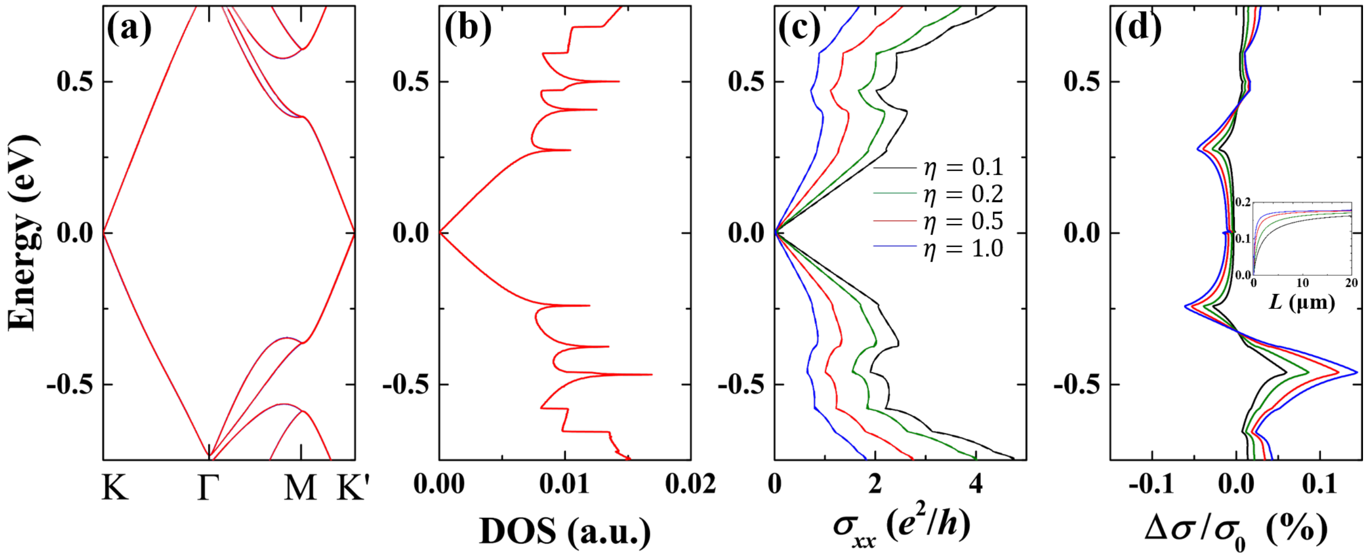


FIG. S3: **At twist angle $\theta$= 6.0°.** (a) Band structure, (b) density of states (DOS), (c) conductivity $\sigma_{xx}$, and (d) relative change of $\sigma_{xx}$ of TBG for **I** || **B** (B=10 T) as functions of energy for fixed length $L = 2\mu$m. In (c)-(d) the black, green, red, and blue lines are calculated under dephasing $\eta = 0.1, 0.2, 0.5$, and 1.0 meV, respectively. The inset in (d) shows the length dependence of the positive peak value under fixed dephasing $\eta = 1$ meV.

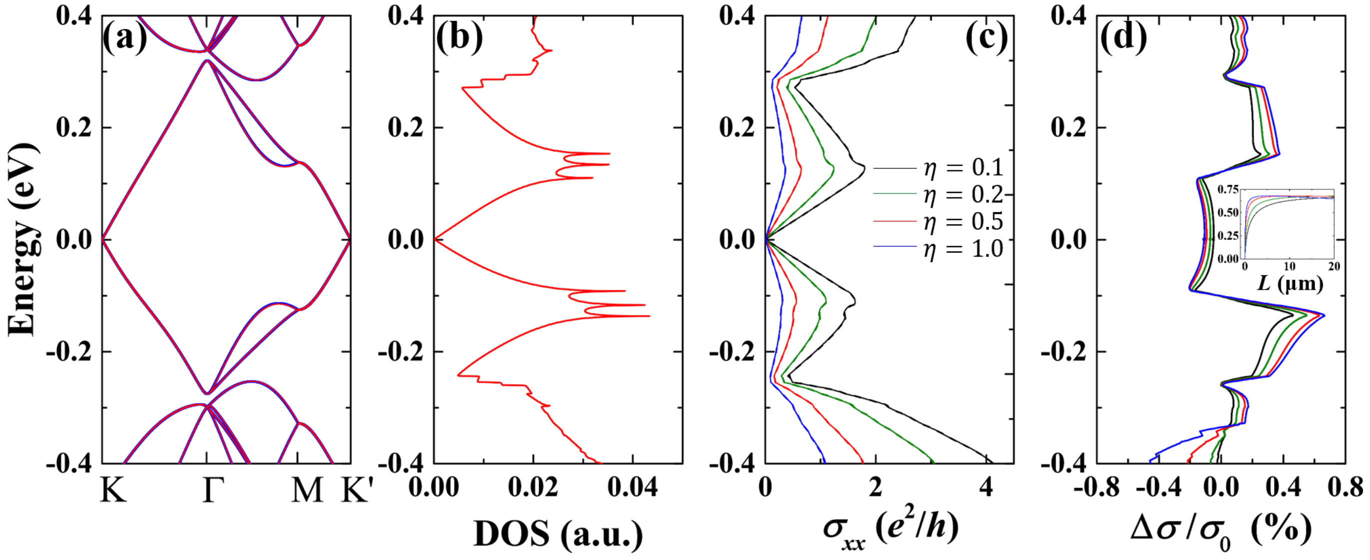


FIG. S4: **At twist angle $\theta$= 3.15°.** (a) Band structure, (b) density of states (DOS), (c) conductivity $\sigma_{xx}$, and (d) relative change of $\sigma_{xx}$ of TBG for **I** || **B** (B=10 T) as functions of energy for fixed length $L = 2\mu$m. In (c)-(d) the black, green, red, and blue lines are calculated under dephasing $\eta = 0.1, 0.2, 0.5$, and 1.0 meV, respectively. The inset in (d) shows the length dependence of the positive peak value under fixed dephasing $\eta = 1$ meV.

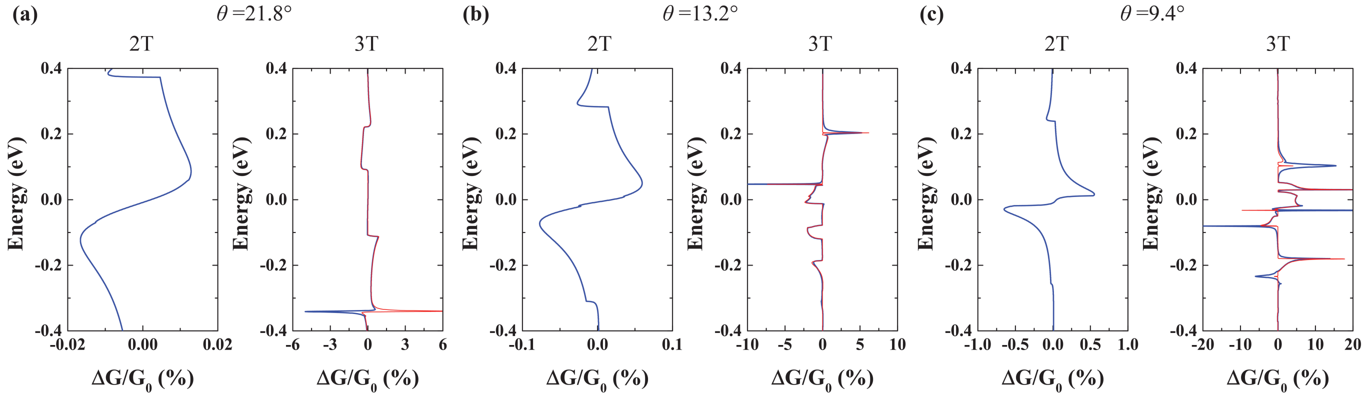


FIG. S5: UMC of two-terminal (2T) and three-terminal (3T) structures for different twist angles: 21.8° (a), 13.2° (b), and 9.4° (c), respectively. For 2T transport a finite dephasing parameter $\eta$ = 10 meV is used; for 3T transport, both $\eta$ = 0 (red) and 10 meV (blue) results are shown.

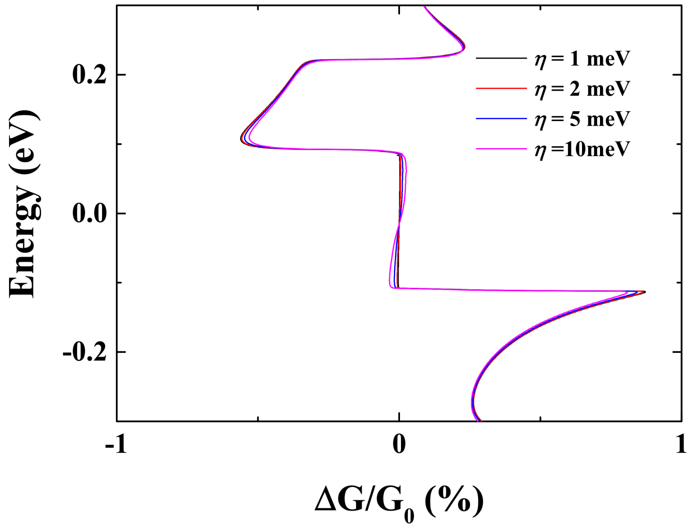


FIG. S6: 3T UMC under different $\eta$ values for twist angle 21.8°.

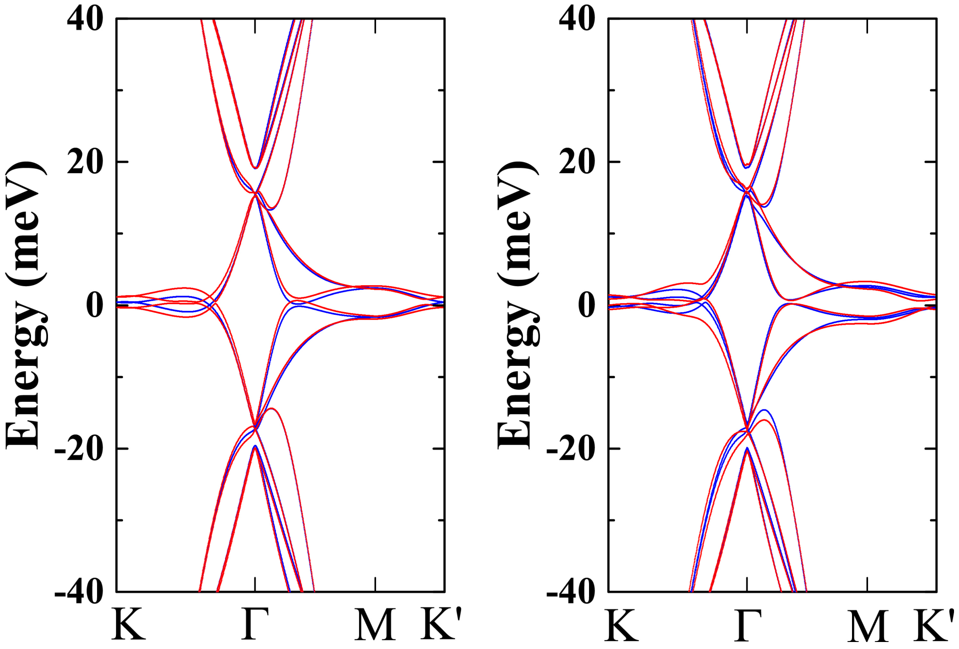


FIG. S7: Band structure of TBG at first magic angle with **I** || **B** (left panel) and **I** ⊥ **B** (right panel), respectively. Blue and red lines refer to $B = 0$ and 10 T, respectively.
